# Supplementary material for: A granular scaling approach to landslide runout
Source: arXiv:2406.14810 ancillary file (2024-06-21)
Supplement: Supplementary file 1 [file landslideFrictionCollapse_SM.pdf]

# A granular scaling approach to landslide runout: Supplementary Material

## CONTENTS


I. Laboratory grain size distributions 2

II. Front speed 3
A. Determining $U$ 3
B. Determining normalization of $U$ 4

III. Alternative normalizations and scaling of diameter 5

IV. Literature data 7
A. Debris flows, landslides 7
B. Volcanic landslides 9
C. Snow avalanches 10
D. Rock avalanches 12
E. Table of field data 16

References 16

# I. LABORATORY GRAIN SIZE DISTRIBUTIONS

Here we provide additional experimental details of the laboratory grains and the determination of their size distributions. Using a weight scale and measuring the volume displaced by a large number of grains, we determine the mass density of all laboratory grains (glass grains from OTS) to be $\rho = 2.48 \pm 0.01$ g/cm$^3$. We determine the size distribution of the grains used in our laboratory experiments by imaging the grains (see Fig. S1a). We sprinkle the grains in between two vertical glass plates and observe them with a steady illumination and fast camera. In this way the particles generally do not touch and we can accurately estimate their size. We fit an ellipse to each grain and defined the diameter $D$ of each grain as the average between the semi-major ($a$) and semi-minor ($b$) axes (see Fig. S1a). We used our own Python scripts that utilize the OpenCV library [1] to process the images to determine $D$. This yields the number-weighted probability distribution $p_{\text{frequency}}(D)$. We confirm this estimate of $p_{\text{frequency}}(D)$ by counting and measuring the total weight of grains on a sensitive scale (Adam Equipment PW 254) and verify that the average diameter determined from $p_{\text{frequency}}(D)$, $\int_0^\infty p_{\text{frequency}}(D)dD$, is within 2% of the estimate from the manual counting method. We then convert the size distributions to the mass-weighted distribution $p(D)$ (see Fig. S1b). Some of the grain distributions were originally bimodal, containing a large amount of relatively small and large grain sizes, which could also have some slight asymmetry or skewness ($S = \langle D^3 \rangle / \langle D \rangle^3 > 1$). We sieved these grains using stainless steel test sieves (VWR) to prepare a more symmetric, nearly gaussian distribution of grain sizes.

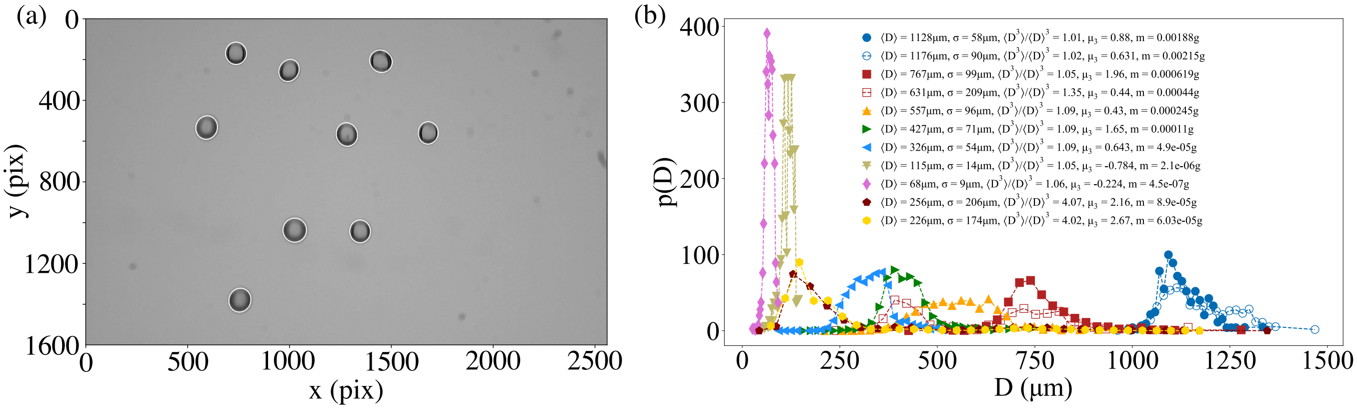


FIG. S1. (a) Example particle images used to determine grain size distributions. The particle size is determined by fitting an ellipse to the grains falling through a narrow gap between two glass plates. These grains correspond to the $\langle D \rangle = 1127$ $\mu$m grain distribution in (b). (b) Plot of grain size distribution weighted by mass (or equivalently by volume). The ratio $S = \langle D^3 \rangle / \langle D \rangle^3$ is also included as well as the normalized skewness $\mu_3$.

## II. FRONT SPEED

### A. Determining $U$

Here we provide additional experimental details of the front speed $U$ discussed and presented in Fig. 2 of the main text. To determine the front speed $U$ in the laboratory experiments, we used a standard image processing tool (ImageJ) to manually track the front position of the landslide. As shown in Fig. S2b, a series of zoomed-in images of near the junction between the inclined and flat section of the experiments, the front is easily distinguished (represented by a black dot). We fit a line to the front positions for the first three time steps after the junction. We estimate $U$ as the slope of this line, and thus $U$ is really an initial front speed since the landslide necessarily decelerates after the junction. We estimated an error bar in this determination of $U$ by the difference between the speed estimated by fitting three or four points.

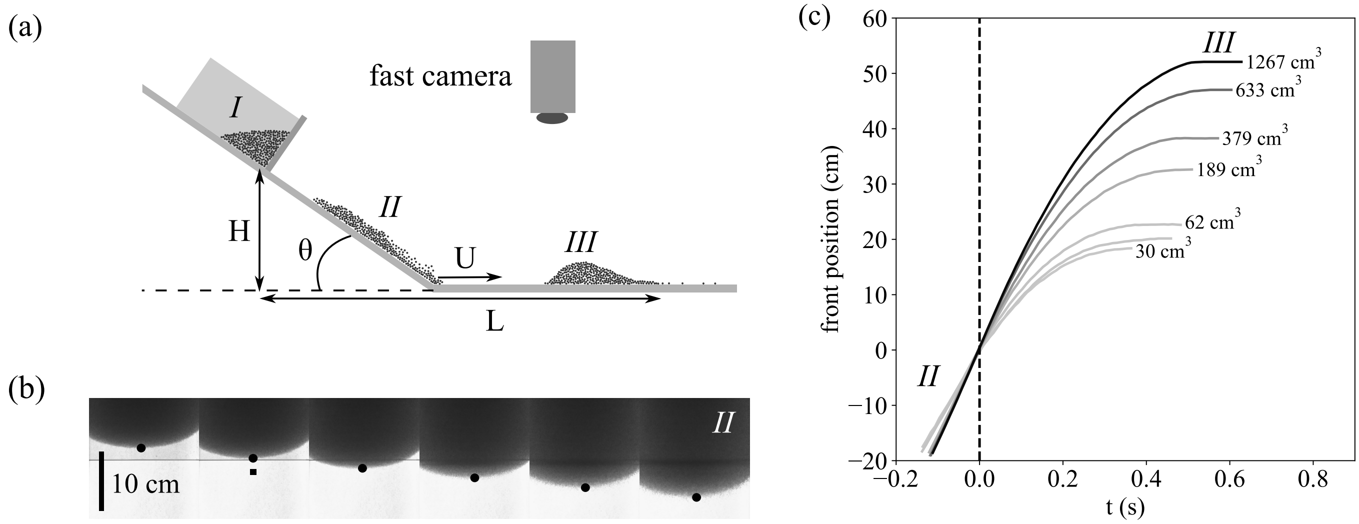


FIG. S2. (a) Side-view schematic of the experimental setup. The grains are released from a rectangular box ($I$) of width 15 cm via a sliding sluice gate at the front and slide down a flat glass plate (80 cm long and 65 cm wide), inclined at an angle $\theta \simeq 34°$, and eventually reach the junction ($II$) before coming to rest on a level flat glass plate (125 cm by 125 cm). The motion of the grains is observed with an overhead fast camera to determine the front speed $U$ at the junction. (b) Representative image series of an experimental granular landslide near the junction (horizontal line in all images) at intermediate times ($II$). Time is from left to right and the flow direction is down. Images are 0.01 s apart. The black dot identifies the front position. Here the total volume is $V \simeq 633$ cm$^3$ ($M \simeq 1000$ g), and the grain size is $\langle D \rangle = 562\mu$m. (c) Time series of front position for several different volumes for the grain size $\langle D \rangle = 328\mu$m. The time $t = 0$ is defined as the moment when the front crosses the junction. Both the slope, from which we determine $U$, and the final distance depend on $V$.

### B. Determining normalization of $U$

Here we show the raw front speed $U$ data for the laboratory experiments and ping-pong experiments [2–4]. The front speeds from the original ping-pong ball experiments were reported as a function of the number of ping-pong balls $N$. The authors argued that the relevant length scale of the system was $L \propto V^{1/3} \propto D_{\text{ping-pong}} N^{1/3}$, where $D_{\text{ping-pong}}$ is the diameter of the ping-pong balls (3.8 cm). In Fig. S3 we show different choices of the length scale for normalizing the front speeds, including the ping-pong ball experimental data. Not normalizing the data yields respectable collapse for the laboratory experiments and ping-pong ball experiments separately (Fig. S3a), but determining what normalization will bring them into accord will yield insights into which parameters are important. Normalizing with $\langle D \rangle$ and $H$ yields even worse collapse, demonstrating that $H$ is not an appropriate length scale for $U$ for this data (Fig. S3b). Including the granularity through $\langle D \rangle$ and $\langle D^3 \rangle$ yields not only better collapse for the laboratory data but also brings the ping-pong ball data into accord as well (Fig. S3c,d). With the ping-pong ball data and for most of our laboratory data, $S \sim 1$, and so we can not determine whether $\langle D^3 \rangle$ or $\langle D \rangle$ should normalize $U$ or $V$. We thus performed additional experiments with mixtures of grains to increase $S$, although this also has the potential to introduce additional effects due to bidispersity [5, 6]. We found that for the front speed $U$, normalizing $U$ with $\langle D^3 \rangle$ and $V$ with $\langle D \rangle^3$ was key to achieving the best collapse of the data (Fig. S3c,d). We thus used this pairing in the main manuscript.

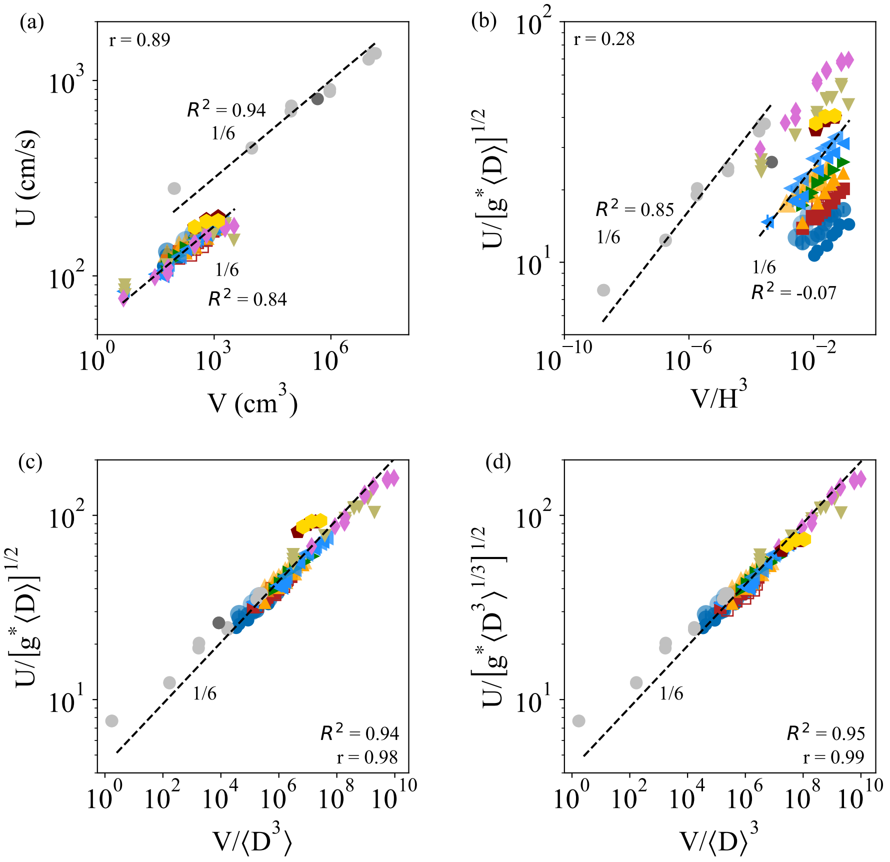


FIG. S3. Alternative plots of normalization for the front speed. All fits (— — —) are to all data with corresponding Spearman correlation coefficients $r$ in each subplot. The goodness of fit ($R^2$) is with respect to the fit. (a) The un-normalized $U$ vs. $V$ shows the $U \propto V^{1/6}$ observed for ping-pong balls (there with $N$ instead of $V$). (b) A plot of normalized front speed using $\langle D \rangle$ and $H$. The collapse is even worse than in (a). (c) A plot of runout speed normalized using the granularity: $U$ is normalized by $\langle D^3 \rangle$ and $V$ by $\langle D^3 \rangle$. The collapse is significantly improved but the data with large $S$ do not collapse well with the rest of the data. (d) A plot of runout speed normalized using the granularity: $U$ is normalized by $\langle D^3 \rangle$ and $V$ by $\langle D \rangle^3$. Now the collapse of the laboratory data is significantly improved and including also the effective gravitational acceleration the ping-pong ball experiments are also in accord. With this normalization the laboratory data with $S \sim 4$ also collapse.

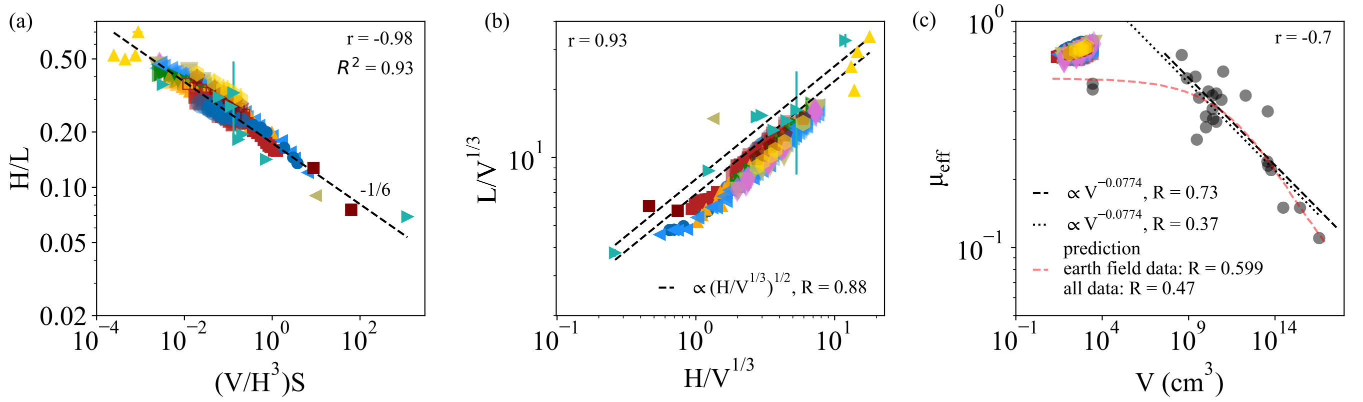


FIG. S4. Alternative plots of runout normalization. All fits (− − −) are to all data with corresponding Spearman correlation coefficients $r$ for all data in each subplot. We sampled laboratory data points evenly (logarithmically) spaced and with a number equal to the field data for the correlation and goodness of fit ($R^2$). (a) Our own normalized runout plot. This is the same as Fig. 3c in the main text. (b) A plot of runout vs. drop height where both are normalized by $V^{1/3}$ [7]. The relative good fit to $(H/V^{1/3})^{1/2}$, apparently unremarked on before now, is equivalent to the dependence of $L$ on $H^{1/2}$ and $V^{1/6}$ seen in Fig. 2c and Fig. 3b in the main text. (c) A plot of a recently proposed effective friction $\mu_{\text{eff}}$, derived from a continuum model [8], vs. $V$. Because their model requires different parameters, we use their field data (terrestrial only) and compare it with our experiments. We compared both the model's fit to just their terrestial data ("earth field data") and to their terrestrial data plus their laboratory data and our own laboratory data ("all data"; our laboratory data was logarithmically spaced in $V$ and with the same number of data points to avoid over-weighting).

## III. ALTERNATIVE NORMALIZATIONS AND SCALING OF DIAMETER

In addition, in Fig. S4 we include plots of several alternative normalizations of the runout from the literature [7, 8]. Fig. S4a is our final normalization from the main text. In Fig. S4b the runout is plotted versus the drop height but with both normalized by $V^{1/3}$ [7]. There is reasonable collapse and the data appear to follow a trend of $(H/V^{1/3})^{1/2}$ (the exponent is not give in Ref. [7]), which is similar to our Fig. 3b in the main text in which we ignore granularity. In Fig. S4c we show a more recently proposed definition of runout friction using a continuum model [8]. Because their model uses the initial thickness as well as the initial span of the landslide deposit, here we used their terrestrial field data (and two experimental data) instead of the field data analyzed by us and used in the main text for which we did not always have access to this information. We do include our experimental data for which we can determine these parameter values. The empirical power law at large $V$, $\mu_{\text{eff}} \propto V^{-0.0774}$, yields a decent fit to the field data but not to the experiments. Their predicted curve improves on this by giving the impression of connecting the experimental and field data. However, the fit is not as good as our own scaling in Fig. S4a and $\mu_{\text{eff}}$ can not account for the clear dependence on the skewness, represented by $S = \langle D^3\rangle/\langle D\rangle^3$, found in our analysis. Moreover while $\mu_{\text{eff}}$ is a decreasing function of $V$ for the field data it is an increasing function for our experiments, which unlike our own scaling suggests that experiments can not be used to make quantitative investigations into the behavior of natural landslides.

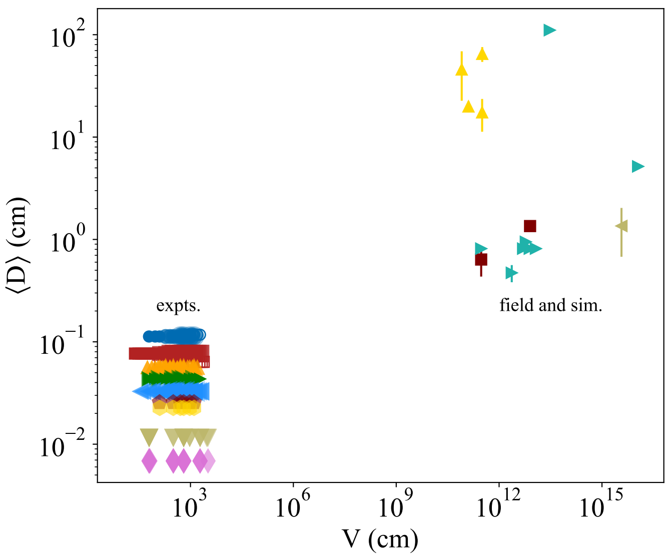


FIG. S5. Comparison of landslide diameters $\langle D\rangle$ vs. total landslide volume $V$. As expected small $\langle D\rangle$ corresponds to small $V$ and large $\langle D\rangle$ corresponds to large $V$, but there is otherwise no noticeable relationship between $\langle D\rangle$ and $V$. This serves to highlight the remarkable collapse of Fig. 3 in the main text.

In Fig. S5 we also make a comparison with the average diameters $\langle D\rangle$ of the data plotted in Fig. 3 in the main text. Besides the expected disparity in size between the small $\langle D\rangle$ for the relatively small $V$ laboratory experiments compared to the large $\langle D\rangle$ for the relatively large $V$ natural data, there does not appear to be any significant correlation. This lack of correlation between $\langle D\rangle$ and $V$ serves to highlight the remarkable collapse furnished by accounting for $\langle D\rangle$ in Fig. 3 in the main text.

## IV. LITERATURE DATA

Here we provide information about where the information about field data or other literature data was found and any essential information or assumptions used in analyzing the data. We use the following protocol for analyzing the grain distributions in the literature. We digitize [9] the granular size distribution from the literature, which is often provided as a cumulative distribution. If not already in the form of $p(D)$, we transform it into this form, which may require re-sampling the data to take the derivative, since the sampled data are usually logarithmically spaced. To re-sample the data we either fit a polynomial to the data (where we take the logarithm of the grain size), or we perform cubic interpolation. Although the two methods do not typically differ by much, attesting to the robustness of our approach, we choose to use the polynomial fitting method. Then we determine $\langle D \rangle$ and $\langle D^3 \rangle$ using the mass-weighted PDF. If the literature source provides a distribution weighted by number, we converted it to a mass-weighted distribution using and then renormalized the distribution to ensure that $\int_0^\infty p(D)dD = 1$ as it must for all probability distributions. We then calculate $\langle D \rangle$ and $\langle D^3 \rangle$ to determine $S = \langle D^3 \rangle / \langle D \rangle^3$ for use in Fig. 3 in the main manuscript, along with information about the landslide volume $V$, runout distance $L$, and fall height $H$ provided in the same literature source or often another source.

### A. Debris flows, landslides

**Debris flows, landslides: Donghekou landslide [10, 12]:**

The 2008 Wenchuan earthquake in Wenchuan County, Sichuan Province, China on 12 May 2008 directly caused a large number of landslides, rockfalls, and debris flows [12]. Granular size distribution data is available for one of these [10], the Donghekou landslide in Qingchuan County. From Yin *et al.* [12] we obtained the landslide front fall height $H = 9.20 \times 10^3$ cm and front travel distance $L = 1.22 \times 10^5$ cm from their cross-section schematic. Yin *et al.* [12] estimated the landslide volume to be $V = 1 \times 10^{13}$ cm$^3$, while Chang *et al.* [10] estimated $V = 6 \times 10^{12}$ cm$^3$, so we took the average of the two estimates $V = 8 \times 10^{12}$ cm$^3$. We obtained a cumulative grain size distribution weighted by mass, $p(D' \leq D)$, from Chang *et al.* [10] who dry-sieved samples of the final landslide pile. We show the original (digitized) data as well as the calculated probability distribution $p(D)$ used to determine $\langle D \rangle = 1.351$ cm and $\langle D^3 \rangle = 15.096$ cm$^3$ in Fig. S6. This yields $S = \langle D^3 \rangle / \langle D \rangle^3 \simeq 6.12$. They were not able to remove all of the moisture from the samples before sieving, but estimate that the maximum dry density, the density that includes all of the solid material as well as the voids, was $\langle \rho_{\mathrm{dry}} \rangle = 1.77$ g/cm$^3$. They also state that the landslide was composed mainly of dolomitic limestone, which has a dry grain material density of $\rho_{\mathrm{mat}} = 2.75$ g/cm$^3$ with a porosity [13] of 1.5%. Thus the packing fraction is $\phi = 1.77/(0.985 \times 2.75) = 0.65$.

**Debris flows, landslides: Chenjiaba landslide [11, 14]:**

The Chenjiaba landslide was induced by heavy rainfall in 2016 in Beichuan County, Sichuan Province, China. (An earlier landslide was also induced at this same location by the Wenchuan earthquake of 2008, but this landslide was partially blocked by a river bed.) From Huang *et al.* [14] we obtained the landslide volume of $V = 3 \times 10^{11}$ cm$^3$, as well as the front fall height $H = 4.96 \times 10^3$ cm and front runout distance $L = 3.90 \times 10^4$ cm from their cross-section schematic. We obtained the grain size distribution from Getahun *et al.* [11], who took samples at various depths and positions of the landslide and dry sieved them to obtain $p(D' \leq D)$. Since the landslide grain sizes were slightly segregated, with larger grains on the top and smaller grains on the bottom, we determined $\langle D \rangle$ and $\langle D^3 \rangle$ for all four depths that they sampled and averaged these values, yielding $\langle \langle D \rangle \rangle_{\mathrm{all}} = 0.637 \pm 0.203$ cm and $\langle \langle D^3 \rangle \rangle_{\mathrm{all}} = 0.912 \pm 0.598$ cm$^3$. This yields $S = \langle D^3 \rangle / \langle D \rangle^3 \simeq 3.54$. We used the variation in the four samples to determine an uncertainty in our estimate of $\langle D \rangle$ and $\langle m \rangle$, which gave us the horizontal and vertical error bars on this data point in the main manuscript. In Fig. S6 we show the distribution from one sample. The composition of the landslide is primarily shale [11], which has a grain material density [15] of $\rho_{\mathrm{mat}} = 2.365$ g/cm$^3$. Getahun *et al.* [11] also give the dry density $\rho_{\mathrm{dry}}$, which we averaged over the four samples to yield $\langle \rho_{\mathrm{dry}} \rangle = 2.018$, which yields a packing fraction of $\phi = \langle \rho_{\mathrm{dry}} \rangle / \rho_{\mathrm{mat}} = 0.853$, which while well above the random close packing (RCP) value for spheres ($\phi_{\mathrm{RCP}} = 0.64$), is not out of the question for polydisperse grain size distributions [16–18].

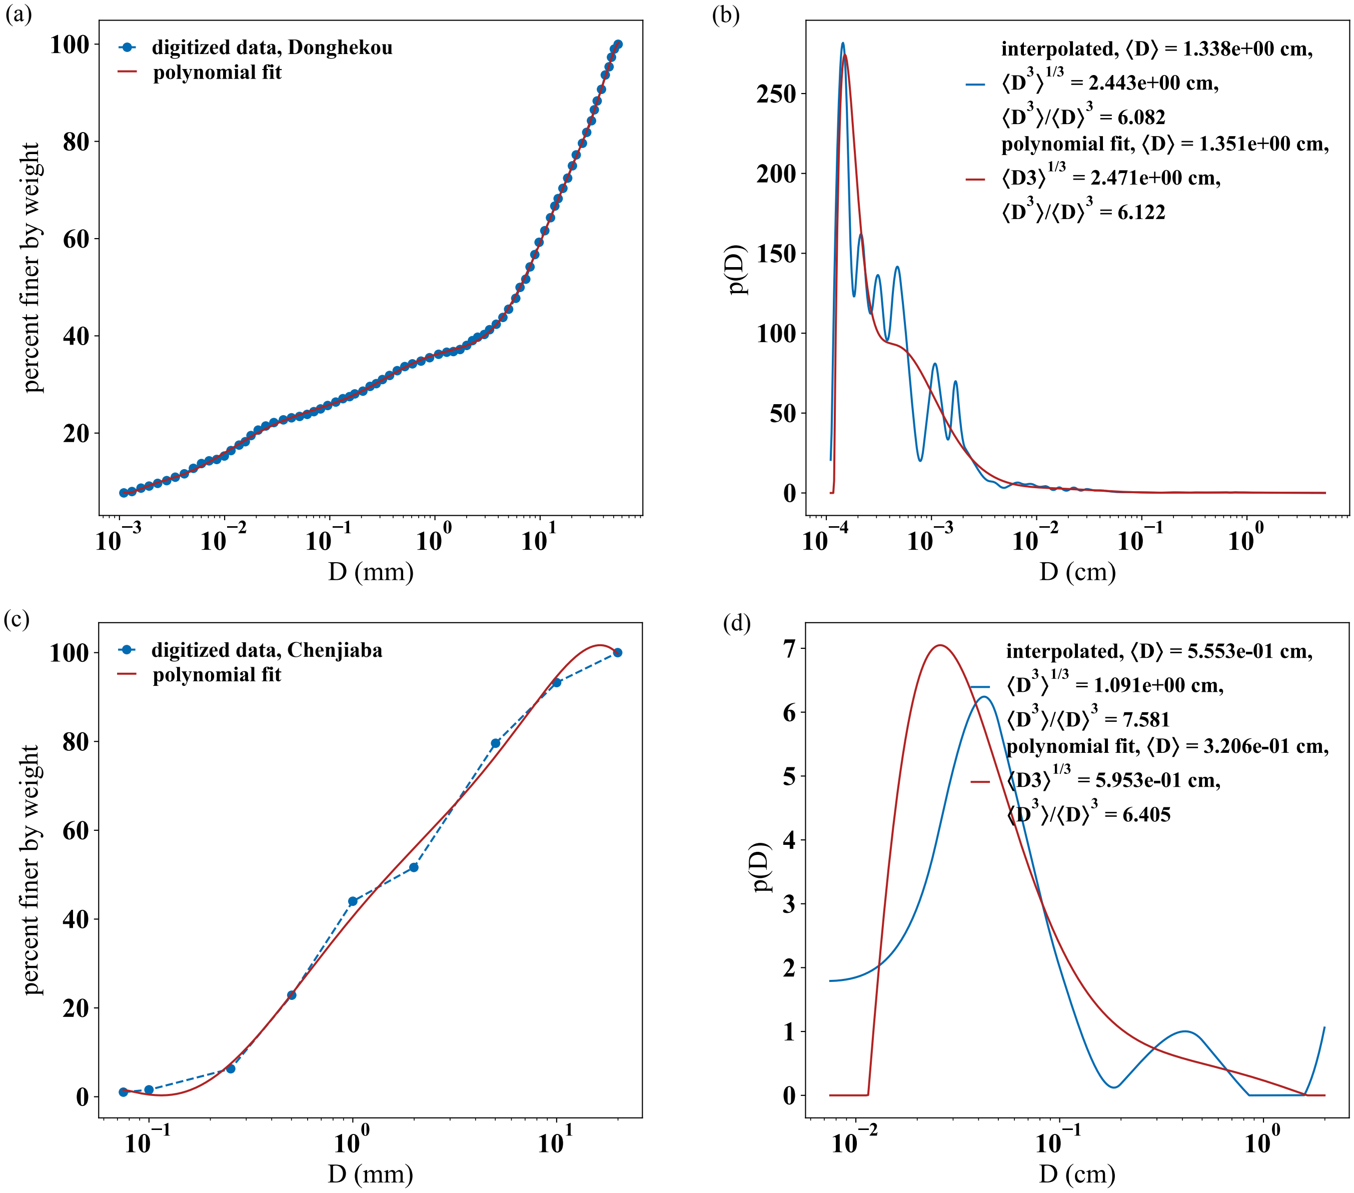


FIG. S6. Plots of digitized and converted grain size distributions for debris flows and landslides. (a) Digitized original data from Chang *et al.* [10]. (b) Mass-weighted probability distribution $p(D)$ determined from original data of (a). (c) Digitized original data from Getahun *et al.* [11]. (d) Mass-weighted probability distribution $p(D)$ determined from original data of (c). The final distribution $p(D)$ is used to determine the mass-weighted average of the diameter $\langle D \rangle$ and the cubed diameter $\langle D^3 \rangle$. Interpolating the non-uniform original data with cubic interpolation or using a polynomial fit yield essentially the same result.

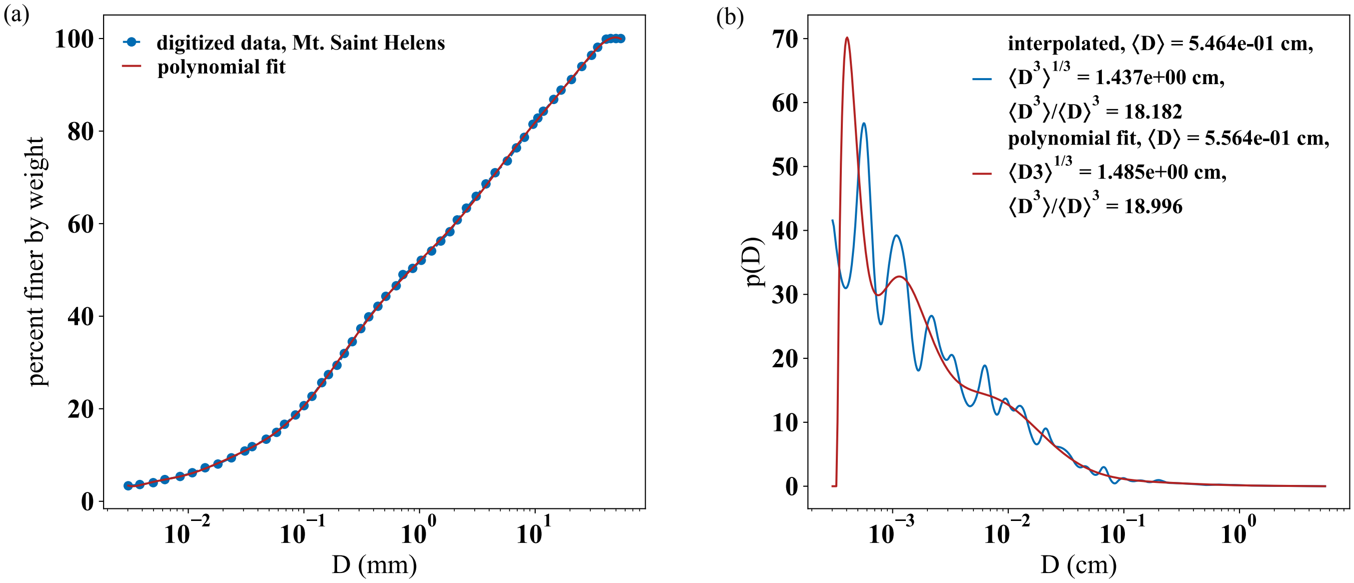


FIG. S7. Plot of digitized and converted grain size distributions for the volcanic landslide. (a) Digitized original data from Voight *et al.* [19] for the Mount Saint Helens volcanic rockslide-avalanche. (b) Mass-weighted probability distribution determined from original data used to determine the mass-weighted average of the diameter $\langle D \rangle$ and the cubed diameter $\langle D^3 \rangle$. Interpolating the non-uniform original data with cubic interpolation or using a polynomial fit yield essentially the same result.

## B. Volcanic landslides

**Volcanic landslides: Mount Saint Helens rockslide-avalanche [19]:**

The earthquake on May 18, 1980 initiated a large mass movement on the slope of Mount Saint Helens, Washington, USA. According to Voight *et al.* [19], the volume of the combined rock and pyroclastic material was $3.706 \times 10^{15}$ cm$^3$, the fall height was $H = 2.070 \times 10^5$ cm, and the runout distance was $L = 2.300 \times 10^6$ cm. Cumulative grain size distributions $p(D' \leq D)$ were determined by sieving several locations [19]. We digitized several distributions (see Fig. S7) and determined ensemble averaged values of $\langle D \rangle = 1.35$ cm and $\langle D^3 \rangle = 58.44$ cm$^3$. This yields $S = \langle D^3 \rangle / \langle D \rangle^3 \simeq 23.54$.

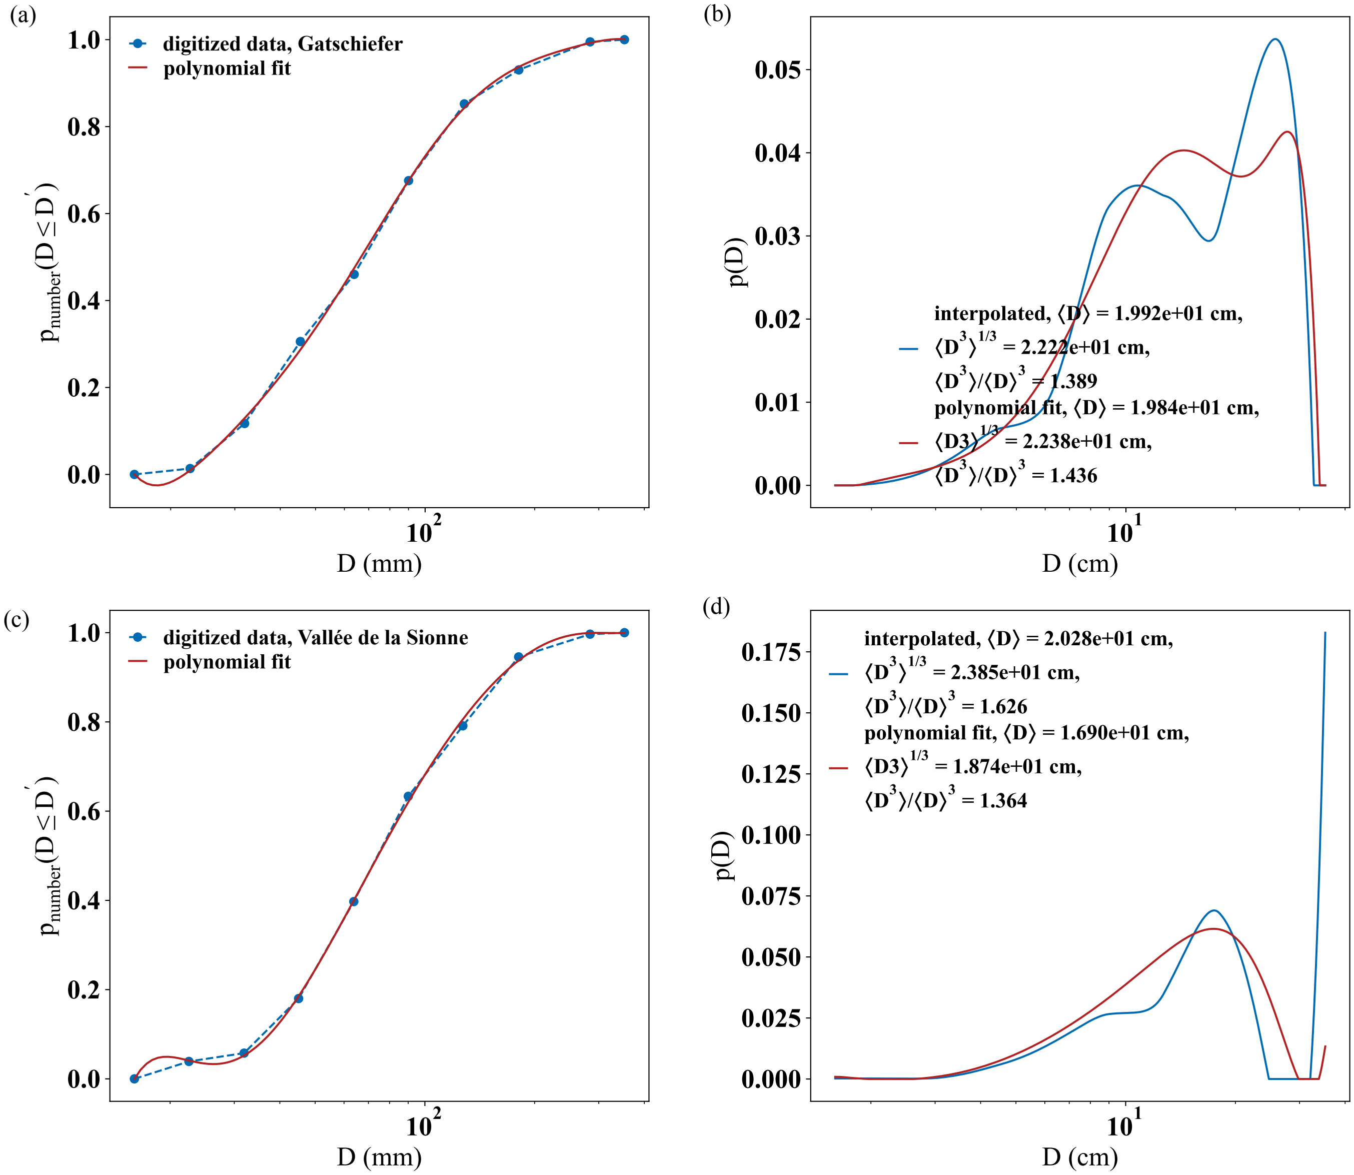


FIG. S8. Plots of digitized and converted grain size distributions for snow and ice avalanches. (a) Digitized original data from Bartelt and McArdell [20] for the snow avalanche at Gatschiefer. (b) Mass-weighted probability distribution determined from original data (a). (c) Digitized original data from Bartelt and McArdell [20] for the snow avalanche at Vallée de la Sionne. (d) Mass-weighted probability distribution determined from original data (c). The final distribution $p(D)$ is used to determine the mass-weighted average of the diameter $\langle D\rangle$ and the cubed diameter $\langle D^3\rangle$. Interpolating the non-uniform original data with cubic interpolation or using a polynomial fit yield essentially the same result.

### C. Snow avalanches

**Snow avalanches: Some artificially-triggered and naturally-triggered snow avalanches [20, 21]:**

The authors measured several samples for each snow avalanche, and we averaged the estimated diameter and mass over the available samples for each avalanche (see an example distribution in Fig. S8). For the four different avalanches studied by Bartelt and McArdell [20], they also gave the estimated volume $V$, fall height $H$, and runout distance $L$. Since the avalanche runout was reported as distance along the slope $L'$, we determined $L = L'/\cos\theta$, where $\theta$ is the slope angle. For some of the snow avalanches, a significant amount of entrainment occurred, whereby the moving snow avalanche accrued more snow as it moved downslope. We use the final volume in our analysis. Below is a table with the parameters from the literature, the average grain diameter and mass, and finally $N$ and $(\langle D\rangle/H)^{1/2}(H/L)$ for each snow avalanche.

| name | wet/dry | $V$ (cm$^3$) | $H$ (cm) | $L$ (cm) | $\langle D \rangle$ (cm) | $\langle D^3 \rangle$ (cm$^3$) | $S = \langle D^3 \rangle / \langle D \rangle^3$ |
|---|---|---|---|---|---|---|---|
| Gatschiefer | wet | $3.22 \times 10^{11}$ | $1 \times 10^5$ | $2.01 \times 10^5$ | 64.94 | $3.77 \times 10^5$ | 1.38 |
| Grünbödeli | wet | $8.12 \times 10^{10}$ | $6 \times 10^4$ | $8.57 \times 10^4$ | 45.73 | $2.94 \times 10^5$ | 2.35 |
| Vallée de la Sionne | dry | $1.28 \times 10^{11}$ | $9 \times 10^4$ | $1.72 \times 10^5$ | 19.90 | $1.11 \times 10^4$ | 1.40 |
| Vallée de la Sionne | dry | $3.20 \times 10^{11}$ | $9 \times 10^4$ | $1.72 \times 10^5$ | 17.42 | $9.19 \times 10^3$ | 1.74 |

## D. Rock avalanches

**Rock avalanches: Mount Cook National Park rock avalanches [22, 23]:**

Rock avalanches frequently occur in the Mount Cook National Park in New Zealand [23]. The two successive Mount Fletcher rock avalanches in 1991 were estimated to have a volume of $V_{\rm I} = 7.8 \times 10^{12}$ cm$^3$ (Mount Fletcher I) and $V_{\rm II} = 5.0 \times 10^{12}$ cm$^3$ (Mount Fletcher II). The volume for these two avalanches was estimated by the volume of water displaced from the lake which they slid into. (Actually, the overflow from this lake entered Lake Tekapo, and the increased volume of Lake Tekapo was used to estimate the additional volume of the unnamed lake, which in turn was used to estimate the rock avalanche volume.) The rock avalanche from Mount Cook also in 1991 had an estimated volume of $V = 1.18 \times 10^{13} \pm 2.4 \times 10^{12}$ cm$^3$. The 1996 Mount Thomson rock avalanche was estimated to have a volume of $V = 3.0 \times 10^{11}$ cm$^3$. According to Fig. 22 in McSaveney [23], the Mount Fletcher I rock avalanche front deposit was initially at $\sim 1948$ m above sea level. The surface of the lake is at $\sim 1056$ m above sea level. Thus the front height fall was determined to be $H_{\rm I} = 8.92 \times 10^4$ cm. The second rock avalanche front deposit was initially at $\sim 1566$ m above sea level, yielding $H_{\rm II} = 5.10 \times 10^4$ cm. The fall height of the Mount Cook avalanche was given as $H = 2.72 \times 10^5$ cm. The front fall height for the Mount Thomson rock avalanche was determined to be $H = 2.43 \times 10^4$ after noting that the rear position was elevated $\sim 700$ m above the final front position, but there was a $\sim 500$ m scar on the $\sim 66°$ slope, which we assume is the scar from the original deposit [23]. The runout distance was determined from the front positions to the beginning of the unnamed lake from Fig. 22 in McSaveney [23], yielding $L_{\rm I} = 2.89 \times 10^5$ cm and $L_{\rm II} = 2.63 \times 10^5$. The runout distance of the Mount Cook rock avalanche was given as $L = 7.5 \times 10^5$ cm. The front runout distance of the Mount Thomson avalanche was estimated to be $L = 8.85 \times 10^4$ cm using the distance from the base of the slope $\sim 600$ m plus the horizontal distance traveled along the slope.

Although the authors provide an empirical fit to the grain size from many different mountains sources [22], this fit (a modified Weibull distribution) does not match the data well at the extreme ends of the empirical distributions and predicts $\langle D^3\rangle^{1/3}/\langle D\rangle \simeq 1$. We thus instead use the empirical grain size distribution from Mt. Cook as representative of the rock avalanches which took place at these three mountains (all in the same geographic location). We digitized the distribution (see Fig. S9) and determined averaged values of $\langle D\rangle = 0.814$ cm and $\langle D^3\rangle = 2.97$ cm$^3$. This yields $S = \langle D^3\rangle/\langle D\rangle^3 \simeq 5.52$.

**Rock avalanches: Flims rock avalanche [24]:**

The Flims rock avalanche is the largest known rock avalanche deposit in Europe [24]. It is believed to have occurred $\sim$ 10,000 years ago on the southern side of the Flimserstein mountain in Switzerland. According to Dunning [24], estimates of its volume range from $1 \times 10^{16}$ cm$^3$ to $12 \times 10^{16}$ cm$^3$, but these larger estimates are based on older maps and we thus take the more recent value of $V = 1.13 \times 10^{16}$ cm$^3$ [25]. The rock avalanche traveled between 7-10 $\times 10^5$ cm from its origin, so we estimated $L = 8.5 \times 10^5$ cm with an uncertainty estimate thus of $\delta L = 1.5 \times 10^5$ cm. The height of the Flimserstein is given as ranging from 1.935 $\times 10^5$ cm to 2.694 $\times 10^5$ cm, so we take the average height of $2.315 \times 10^5$ cm. However, this is the maximum height. The cliff-line, which corresponds to the front position of the original deposit, is estimated to be $5 \times 10^4$ cm below this [24]. The final height of the deposit is estimated to be $1.236 \times 10^5$ cm, resulting in a total height difference of $H = 2.315 \times 10^5 - 5 \times 10^4 - 1.236 \times 10^5 = 5.875 \times 10^4$ cm. The grain material density of the rock was determined to be $\rho_{\rm mat} = 2.53$ g/cm$^3$ [26]. Dunning [24] provided the weight-averaged probability density from several sites (see Fig. S9b for an example) which we used to determine the average diameters and masses. We averaged the results from three different sample sites to determine $\langle D\rangle = 5.17$ cm and $\langle D^3\rangle = 2970$ cm$^3$. This yields $S = \langle D^3\rangle/\langle D\rangle^3 \simeq 21.50$.

**Rock avalanches: Acheron rock avalanche [24]:**

The Acheron rock avalanche occurred $\sim$ 500 years ago in the southern end of the Cragiebum Range, Canterbury, New Zealand [24]. The volume has been estimated from aerial photographs to be $V = 6 \times 10^{12}$ cm$^3$. The deposit scar is apparently clearly distinguishable, with a lower height of $1.3 \times 10^5$ cm. The lowest point of the deposit is at $\sim 8 \times 10^4$ cm, yielding $H = 5 \times 10^4$ cm. From the topographic map in Fig. 6.1 in Dunning [24] we determined $L = 2.748 \times 10^5$. We determined [26] $\rho_{\rm mat} = 2.68$ g/cm$^3$ and estimated $\phi = 0.634$ from similar avalanches in this region [27]. Although the size distributions provided in Dunning [24] appeared to be truncated for diameters larger than 1 cm, even though images of the rock avalanche deposit clearly indicate that there were rocks of larger size, a more complete distribution was provided in McSaveney and Davies [22]. We used this distribution (see Fig. S9e) to determine the average $\langle D\rangle = 0.947$ cm and $\langle D^3\rangle = 3.00$ cm$^3$. This yields $S = \langle D^3\rangle/\langle D\rangle^3 \simeq 3.53$, which is still similar to the value estimated from the incomplete distributions.

**Rock avalanches: Frank rockslide [28, 29]:**

The Frank Slide rock avalanche of 1903 occurred in south-west Alberta (Canada). The volume has been estimated to be $V = 3 \times 10^{13}$ cm$^3$. An early survey provides sufficient information to determine the front drop and horizontal

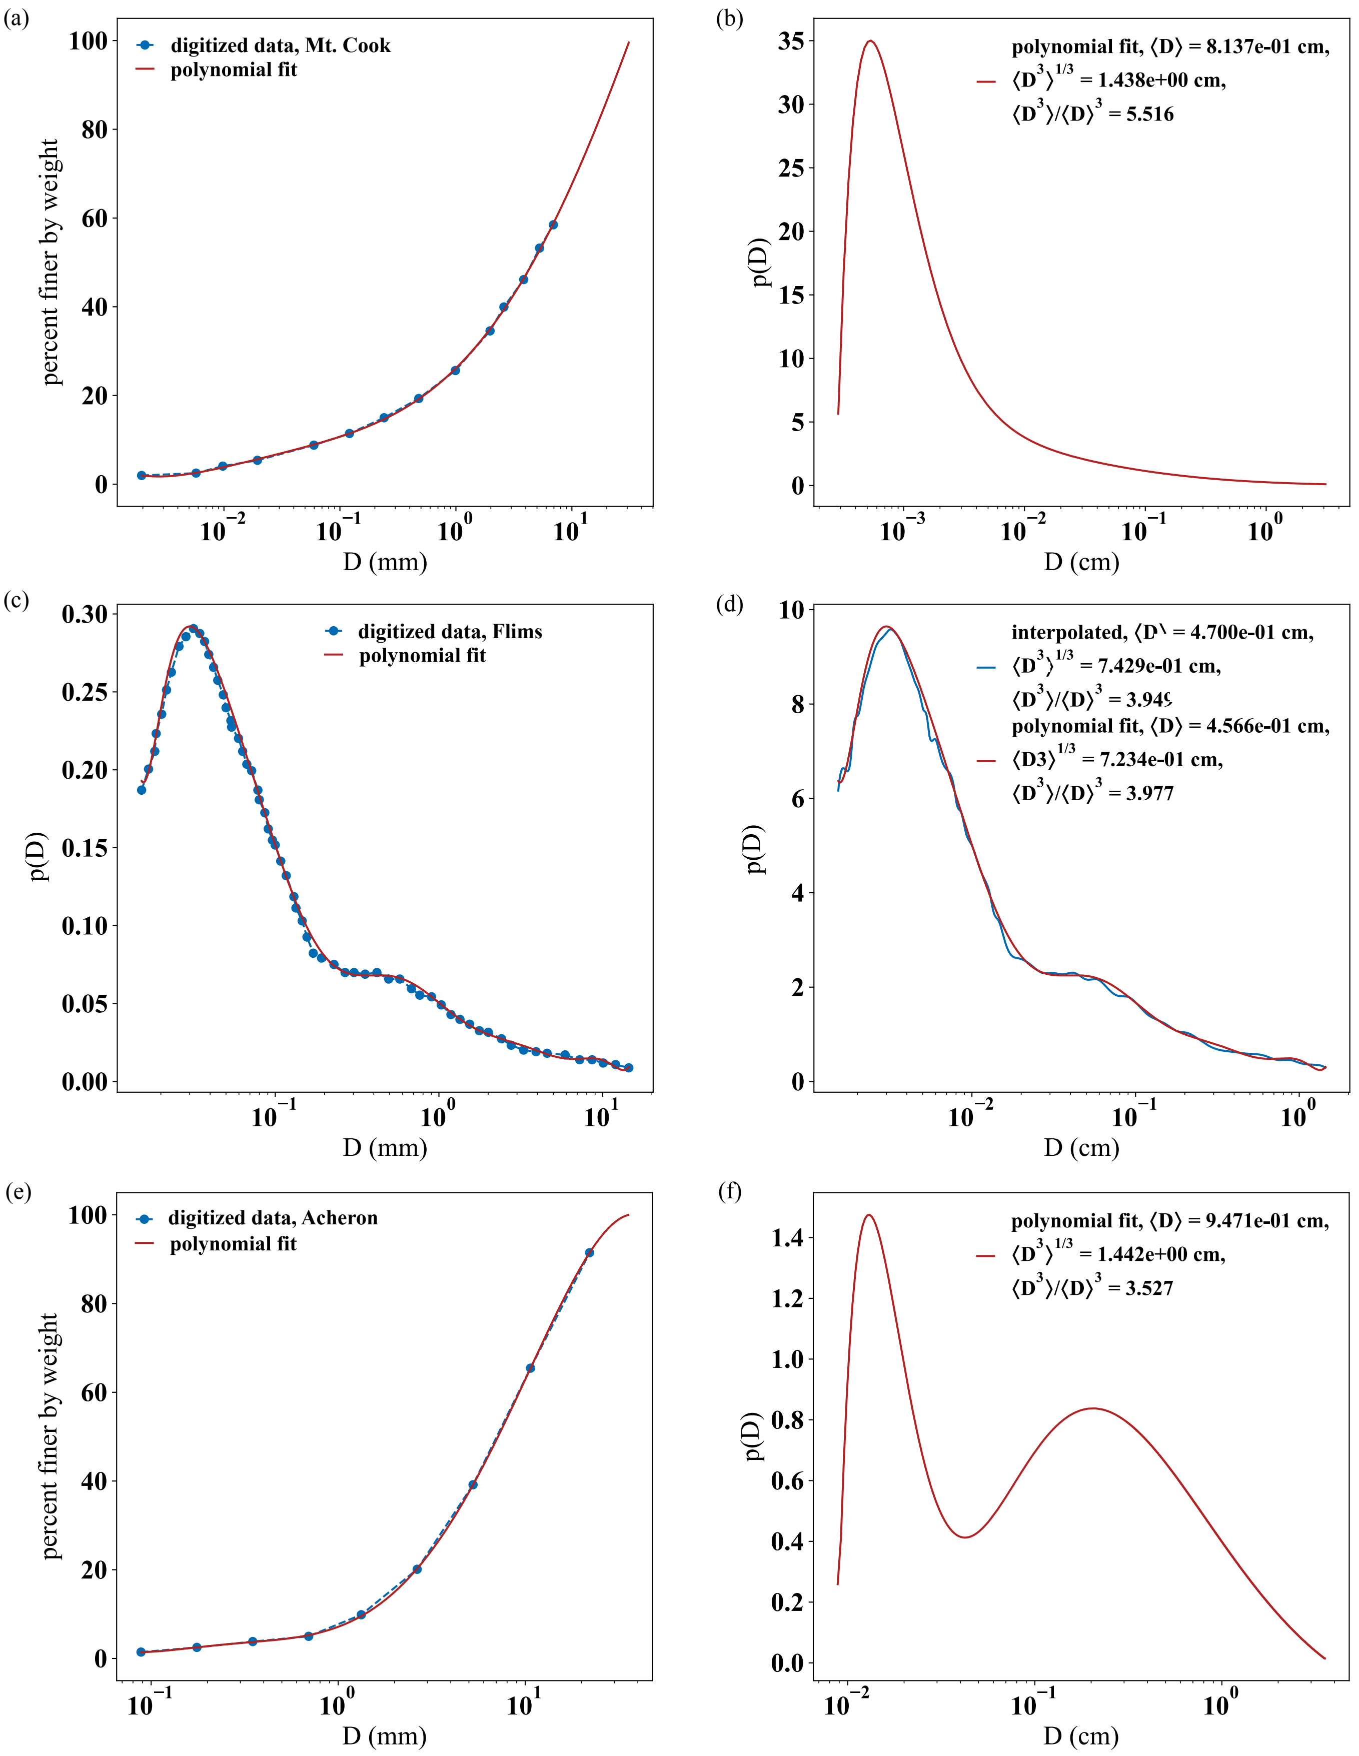


FIG. S9. Plots of digitized and converted grain size distributions for Flims and Acheron rock avalanches. (a),(c),(e) Digitized original data from McSaveney and Davies [22] and Dunning [24] for the Mt. Cook avalanches (a), Flims rock avalanche (c), and Acheron avalanche (e). (b),(d),(f) Mass-weighted probability distribution determined from original data. For (b) the data were already in the form needed for our calculations but still needed to be re-sampled so as to be evenly spaced. The final distribution $p(D)$ is used to determine the mass-weighted average of the diameter $\langle D \rangle$ and the cubed diameter $\langle D^3 \rangle$. Interpolating the non-uniform original data with cubic interpolation or using a polynomial fit yield essentially the same result.

travel distance as $H = 3.850 \times 10^4$ cm and $L = 2.714 \times 10^5$ cm respectively [29]. The material is a mixture of shale, sandstone, siltstone, and dolomite, for which we estimate [30] $\rho_{\text{mat}} = 2.425$ g/cm$^3$. Size distribution data were determined by Charrière *et al.* [28]. Averaging of the results from digitizing and analyzing the two size distributions provided [28] (see Fig. S10), we determined $\langle D \rangle = 111$ cm and $\langle D^3 \rangle = 1.88 \times 10^6$ cm$^3$. This yields $S = \langle D^3 \rangle / \langle D \rangle^3 \simeq 1.38$.

**Rock avalanches: Cayley rockslide [31, 32]:**

A major rock slide occurred on Mount Cayley, British Columbia, Canada, in 1984. The rock slide eventually triggered a debris flow which ran out a comparable distance. Perhaps owing to the increased complexity due to this second event, estimates of the size and extent of the rock avalanche differ substantially [31, 32]. We took the average of the estimates from these two sources and took the grain size distribution from Evans *et al.* [31], which did not appear to differ from the grain size distribution measurements of Cruden and Lu [32]. The volume is thus estimated to be $V = 2.34 \times 10^{12}$ cm$^3$, $H = 7.05 \times 10^4$ cm, and $L = 2.16 \times 10^5$ cm. The pyroclastic material is apparently very porous [32], yielding an estimate $\rho_{\text{mat}} = 0.8896$ g/cm$^3$. Size distribution data were determined by Evans *et al.* [31]. Averaging of the results from digitizing and analyzing the two size distributions provided [31] (see Fig. S10), we determined $\langle D \rangle = 0.4717$ cm and $\langle D^3 \rangle = 2.06$ cm$^3$. This yields $S = \langle D^3 \rangle / \langle D \rangle^3 \simeq 19.59$.

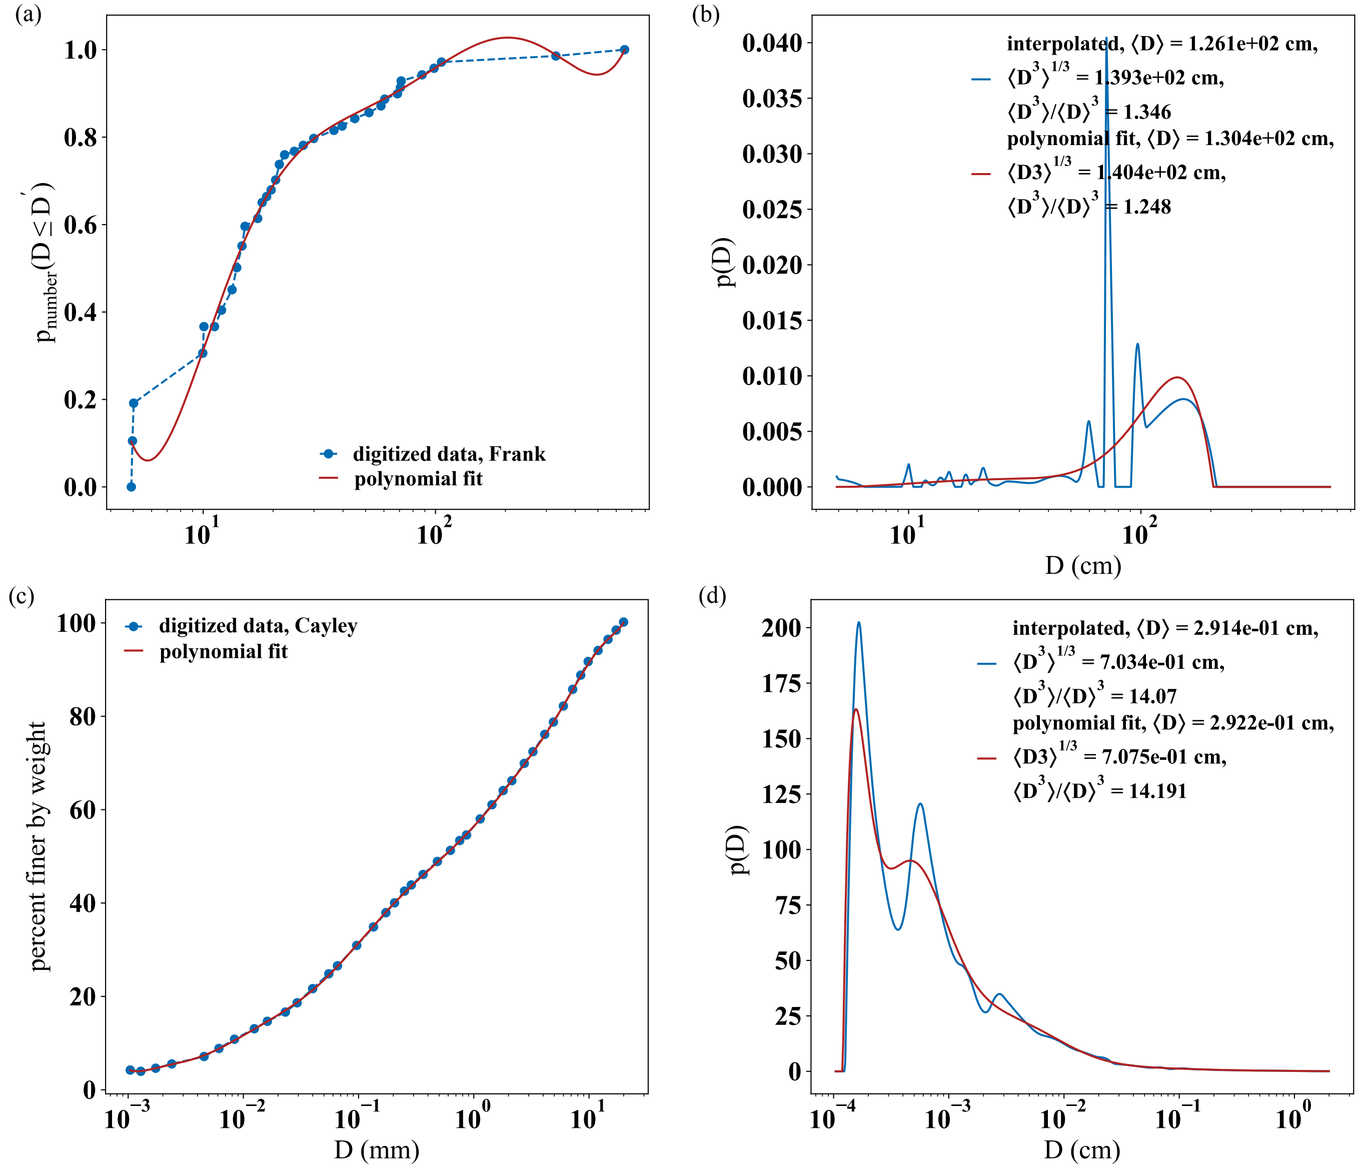


FIG. S10. Plots of digitized and converted grain size distributions for Frank and Cayley rockslides. (a) Digitized original data from Charrière *et al.* [28] for Frank rockslide. (b) Mass-weighted probability distribution $p(D)$ determined from original data of (a). (c) Digitized original data from Evans *et al.* [31] for Cayley rockslide. (d) Mass-weighted probability distribution $p(D)$ determined from original data of (d). The final distribution $p(D)$ is used to determine the mass-weighted average of the diameter $\langle D \rangle$ and the cubed diameter $\langle D^3 \rangle$. Interpolating the non-uniform original data with cubic interpolation or using a polynomial fit yield essentially the same result.

### E. Table of field data

Here we provide a table summarizing the field data used in this work.

TABLE I. Summary of field data.

| Name | $V$ | $H$ | $L$ | $\langle D\rangle$ | $\langle D^3\rangle$ | $\sigma$ | $\mu_3$ (skewness) | Category |
|---|---|---|---|---|---|---|---|---|
| Chenjiaba | 3.00E+11 | 4.96E+03 | 3.90E+04 | 6.37E-01 | 9.12E-01 | 4.84E-01 | 7.27E-01 | dry debris flows |
| Donghekou | 8.00E+12 | 9.20E+03 | 1.22E+05 | 1.35E+00 | 1.51E+01 | 1.50E+00 | 1.04E+00 | dry debris flows |
| Gatschiefer | 3.22E+11 | 1.00E+05 | 2.01E+05 | 6.49E+01 | 3.77E+05 | 2.13E+01 | -7.70E-01 | snow avalanches |
| Grunbodeli | 8.12E+10 | 6.00E+04 | 8.57E+04 | 4.57E+01 | 2.25E+05 | 1.65E+01 | -5.51E-01 | snow avalanches |
| Vallee de la Sionne | 1.28E+11 | 9.00E+04 | 1.72E+05 | 1.99E+01 | 1.11E+04 | 6.95E+00 | -4.23E-01 | snow avalanches |
| Vallee de la Sionne | 3.20E+11 | 9.00E+04 | 1.72E+05 | 1.74E+01 | 9.19E+03 | 5.22E+00 | -4.00E-01 | snow avalanches |
| Mount Fletcher I | 7.80E+12 | 8.92E+04 | 2.89E+05 | 8.14E-01 | 2.97E+00 | 8.57E-01 | 2.47E+00 | rock avalanches |
| Mount Fletcher II | 5.00E+12 | 5.10E+04 | 2.62E+05 | 8.14E-01 | 2.97E+00 | 8.57E-01 | 2.47E+00 | rock avalanches |
| Mount Thomson | 3.00E+11 | 2.43E+04 | 8.85E+04 | 8.14E-01 | 2.97E+00 | 8.57E-01 | 2.47E+00 | rock avalanches |
| Mount Cook | 1.18E+13 | 2.72E+05 | 7.50E+05 | 8.14E-01 | 2.97E+00 | 8.57E-01 | 2.47E+00 | rock avalanches |
| Flims | 1.13E+16 | 5.88E+04 | 8.50E+05 | 5.17E+00 | 2.97E+03 | 3.66E+00 | 7.79E-01 | rock avalanches |
| Acheron | 6.00E+12 | 5.00E+04 | 2.75E+05 | 9.47E-01 | 3.00E+00 | 7.68E-01 | 3.92E+00 | rock avalanches |
| Cayley | 2.34E+12 | 7.05E+04 | 2.16E+05 | 4.72E-01 | 2.06E+00 | 7.12E-01 | 1.77E+00 | rock avalanches |
| Frank | 3.00E+13 | 3.85E+04 | 2.71E+05 | 1.11E+02 | 1.88E+06 | 3.41E+01 | -5.38E-01 | rock avalanches |
| Mount Saint Helens | 3.71E+15 | 2.07E+05 | 2.30E+06 | 1.35E+00 | 5.84E+01 | 1.68E+00 | 1.65E+00 | volcanic landslides |


[1] G. Bradski, The OpenCV Library, Dr. Dobb's Journal of Software Tools (2000).

[2] J. McElwaine and K. Nishimura, Ping-pong ball avalanche experiments, Ann. Glaciol. **32**, 241 (2001).

[3] K. Nishimura, S. Keller, J. McElwaine, and Y. Nohguchi, Ping-pong ball avalanche at a ski jump, Granular matter **1**, 51 (1998).

[4] K. Kosugi, A. Sato, O. Abe, Y. Nohguchi, Y. Yamada, K. Nishimura, and K. Izumi, Table tennis ball avalanche experiments, in *ISSW94 Proceedings, International Snow science Workshop, October 30-November*, Vol. 3 (1995) pp. 636–642.

[5] E. Linares-Guerrero, C. Goujon, and R. Zenit, Increased mobility of bidisperse granular avalanches, Journal of Fluid Mechanics **593**, 475 (2007).

[6] F. Moro, T. Faug, H. Bellot, and F. Ousset, Large mobility of dry snow avalanches: Insights from small-scale laboratory tests on granular avalanches of bidisperse materials, Cold Regions Science and Technology **62**, 55 (2010).

[7] T. Davies and M. McSaveney, Runout of dry granular avalanches, Can. Geotech. J. **36**, 313 (1999).

[8] A. Lucas, A. Mangeney, and J. P. Ampuero, Frictional velocity-weakening in landslides on earth and on other planetary bodies, Nat. Commun. **5**, 1 (2014).

[9] A. Rohatgi, Webplotdigitizer: Version 4.4 (2020).

[10] D. Chang, L. Zhang, Y. Xu, and R. Huang, Field testing of erodibility of two landslide dams triggered by the 12 may wenchuan earthquake, Landslides **8**, 321 (2011).

[11] E. Getahun, S.-w. Qi, S.-f. Guo, Y. Zou, and N. Liang, Characteristics of grain size distribution and the shear strength analysis of chenjiaba long runout coseismic landslide, J. Mt. Sci. **16**, 2110 (2019).

[12] Y. Yin, F. Wang, and P. Sun, Landslide hazards triggered by the 2008 wenchuan earthquake, sichuan, china, Landslides **6**, 139 (2009).

[13] G. E. Manger *et al.*, Porosity and bulk density of sedimentary rocks, Bull. US. Geol. Surv. **1144-E**, 1 (1963).

[14] T. Huang, M.-t. Ding, T. She, S.-j. Tian, and J.-t. Yang, Numerical simulation of a high-speed landslide in chenjiaba, beichuan, china, J. Mt. Sci. **14**, 2137 (2017).

[15] J. S. Moore, X. Prat-Resina, T. Wendorff, A. Hahn, E. Vitz, and J. W., Density of Rocks and Soils (2020), [Online; accessed 2021-03-23].

[16] B. Andreotti, Y. Forterre, and O. Pouliquen, *Granular media: between fluid and solid* (Cambridge University Press, 2013).

[17] R. McGeary, Mechanical packing of spherical particles, J. Am. Ceram. Soc. **44**, 513 (1961).

[18] H. Brouwers, Particle-size distribution and packing fraction of geometric random packings, Phys. Rev. E **74**, 031309 (2006).

[19] B. Voight, R. Janda, H. Glicken, and P. Douglass, Nature and mechanics of the mount st helens rockslide-avalanche of 18 may 1980, Geotechnique **33**, 243 (1983).

[20] P. Bartelt and B. W. McArdell, Granulometric investigations of snow avalanches, J. Glaciol. **55**, 829 (2009).

[21] B. Sovilla, P. Burlando, and P. Bartelt, Field experiments and numerical modeling of mass entrainment in snow avalanches, J. Geophys. Res. Earth Surface **111** (2006).

[22] M. McSaveney and T. Davies, Rockslides and their motion, in *Progress in Landslide Science* (Springer, 2007) pp. 113–133.

[23] M. McSaveney, Recent rockfalls and rock avalanches in mount cook national park, new zealand, in *Catastrophic Landslides: Effects, Occurrence, and Mechanisms*, Vol. 15 (Reviews in Engineering Geology, 2002) pp. 35–70.

[24] S. A. Dunning, *Rock avalanches in high mountains*, Ph.D. thesis, University of Bedfordshire (2004).
[25] O. A. Pfiffner, The flims rock avalanche: structure and consequences, Swiss Journal of Geosciences **115**, 1 (2022).
[26] S. Homuth, A. Götz, and I. Sass, Reservoir characterization of the upper jurassic geothermal target formations (molasse basin, germany): role of thermofacies as exploration tool, Geotherm. Energy Sci. **3**, 41 (2015).
[27] S. Cox and S. Allen, Vampire rock avalanches of january 2008 and 2003, southern alps, new zealand, Landslides **6**, 161 (2009).
[28] M. Charrière, F. Humair, C. Froese, M. Jaboyedoff, A. Pedrazzini, and C. Longchamp, From the source area to the deposit: Collapse, fragmentation, and propagation of the frank slide, Geol. Soc. Am. Bull. **128**, 332 (2016).
[29] W. V. Gassen and D. Cruden, Momentum transfer and friction in the debris of rock avalanches, Can. Geotech. J. **26**, 623 (1989).
[30] B. Benko and D. Stead, The frank slide: a reexamination of the failure mechanism, Can. Geotech. J. **35**, 299 (1998).
[31] S. G. Evans, O. Hungr, and J. J. Clague, Dynamics of the 1984 rock avalanche and associated distal debris flow on mount cayley, british columbia, canada; implications for landslide hazard assessment on dissected volcanoes, Eng. Geol. **61**, 29 (2001).
[32] D. Cruden and Z. Lu, The rockslide and debris flow from mount cayley, bc, in june 1984, Can. Geotech. J. **29**, 614 (1992).
